# Supplementary material for: Electronic Excitations Through the Prism of Mean-Field Decomposition Techniques
Source: arXiv:2112.09508 ancillary file (2022-02-11)
Supplement: Supplementary file 1 [file si.pdf]

# Supporting Information: Electronic Excitations Through the Prism of Mean-Field Decomposition Techniques

Janus J. Eriksen*

*DTU Chemistry, Technical University of Denmark*

*Kemitorvet Bldg. 206, DK–2800 Kgs. Lyngby, Denmark*

E-mail: janus@kemi.dtu.dk

# 1 Separated $F_2 \cdots NH_3$ System

**Table S1:** Individual contributions (in units of $E_H$) to the total excitation energy of the CT transition in the separated $F_2 \cdots NH_3$ system, cf. Fig. 1 or main study.

| Molecule | Coulomb | Kinetics | Nuc. At. (G) | Nuc. At. (L) | Exchange | *xc* |
|---|---|---|---|---|---|---|
| | | | HF | | | |
| $F_2$ | 8.458714 | 1.023584 | −4.520405 | −4.527808 | −0.479558 | — |
| $NH_3$ | −4.076613 | −0.233848 | 2.198904 | 2.206307 | 0.247242 | — |
| | | | B3LYP | | | |
| $F_2$ | 7.749905 | 0.814287 | −4.097096 | −4.104499 | −0.080464 | −0.336815 |
| $NH_3$ | −4.060832 | −0.264402 | 2.206596 | 2.213999 | 0.049200 | 0.252322 |
| | | | CAM-B3LYP | | | |
| $F_2$ | 7.846347 | 0.843270 | −4.155269 | −4.162672 | −0.149408 | −0.283331 |
| $NH_3$ | −4.066645 | −0.261646 | 2.207772 | 2.215175 | 0.113601 | 0.191928 |
| | | | M06-2X | | | |
| $F_2$ | 8.076376 | 0.869257 | −4.272435 | −4.279838 | −0.236235 | −0.207910 |
| $NH_3$ | −4.081493 | −0.265505 | 2.216306 | 2.223709 | 0.134611 | 0.169943 |

# 2 Approximate Spin-Projection

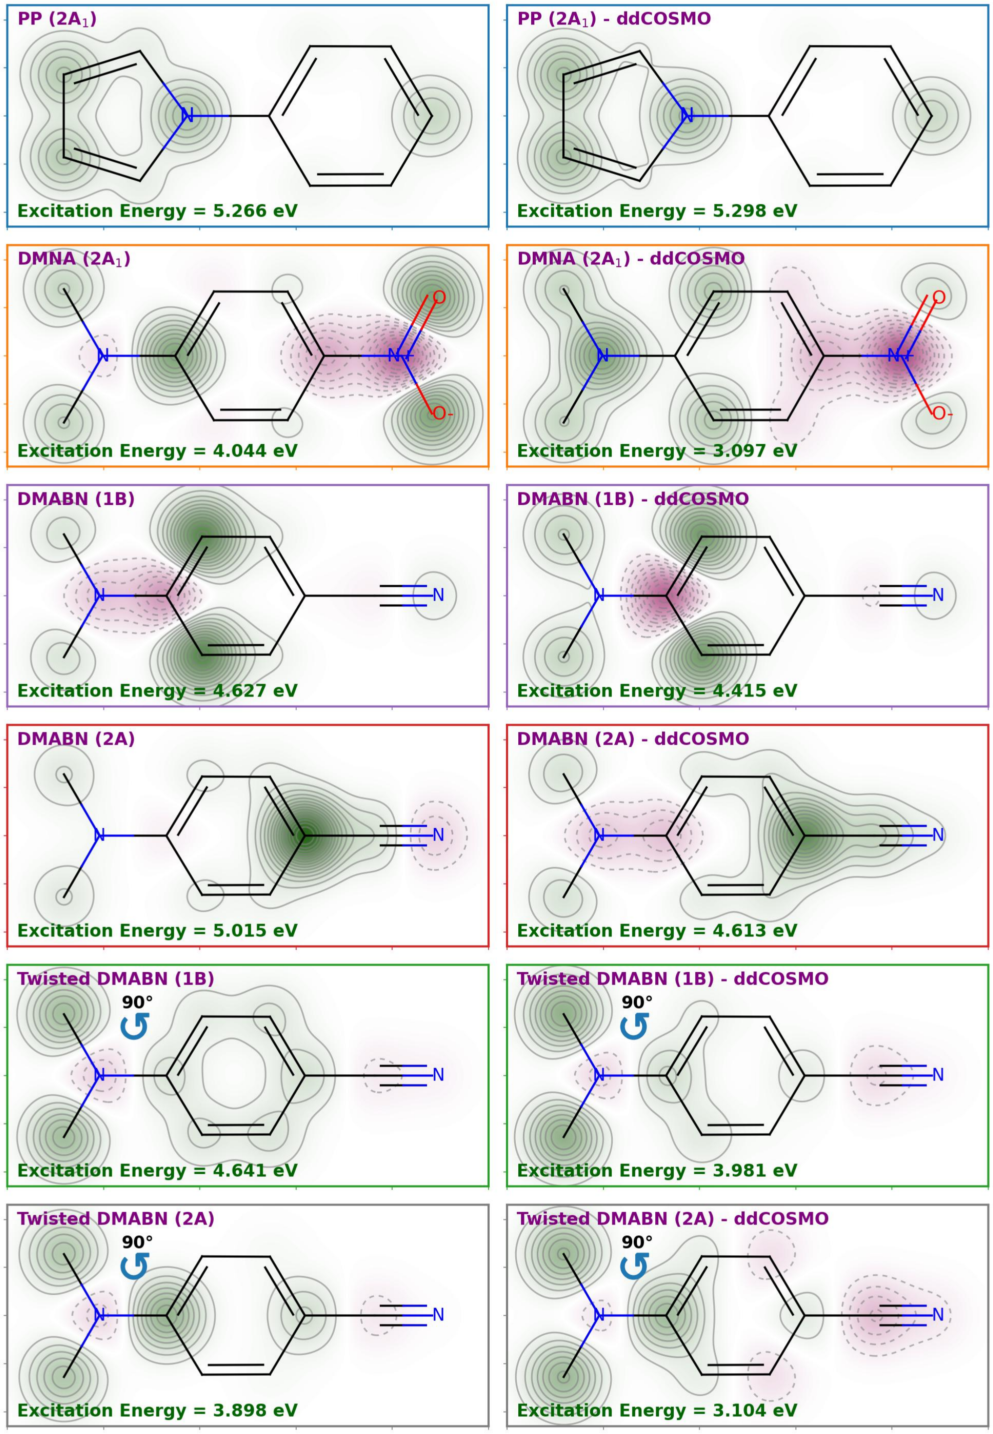


**Figure S1:** Same set of results as in Fig. 2 of main study, but subject to approximate spin-projection. In all plots, pink and green colors indicate negative and positive shifts, respectively, and the plots have been normalized across all individual transitions.

# 3 Localization Procedure

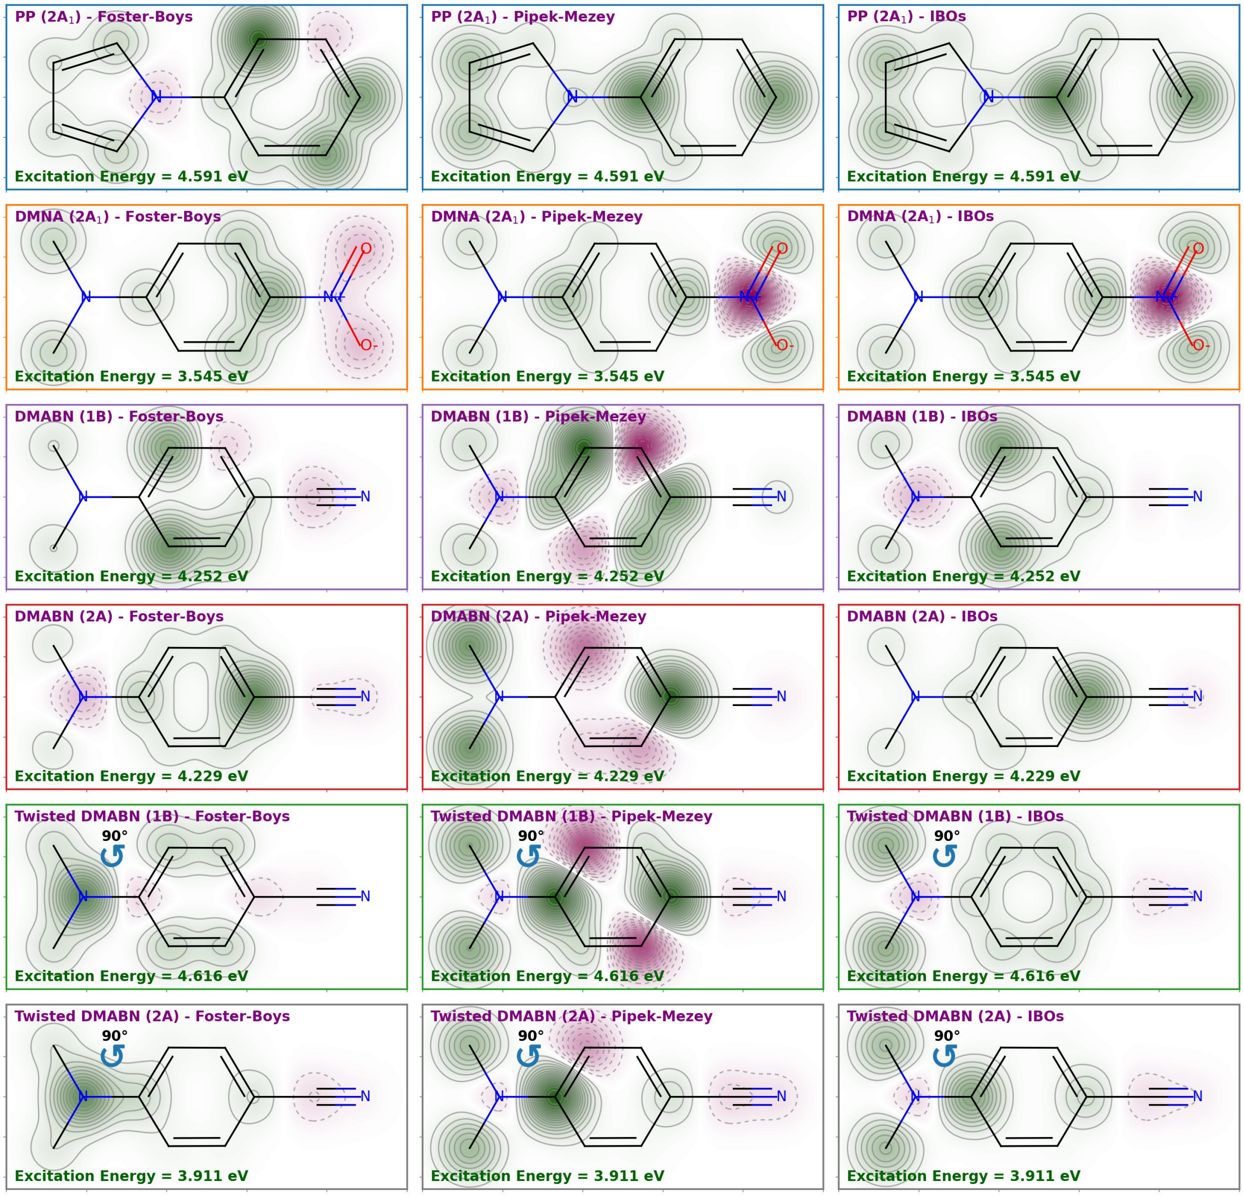


**Figure S2:** Total changes in individual atomic electronic energy contributions along the studied transitions in PP, DMNA, and (twisted) DMABN (in vacuo), as calculated at the CAM-B3LYP/aug-pc-1 level of theory, IAOs, and different sets of localized MOs. The colormap is the same as in Fig. S1, and the plots have been (row-wise) normalized for each of the individual transitions.

# 4 Density Functional Approximation

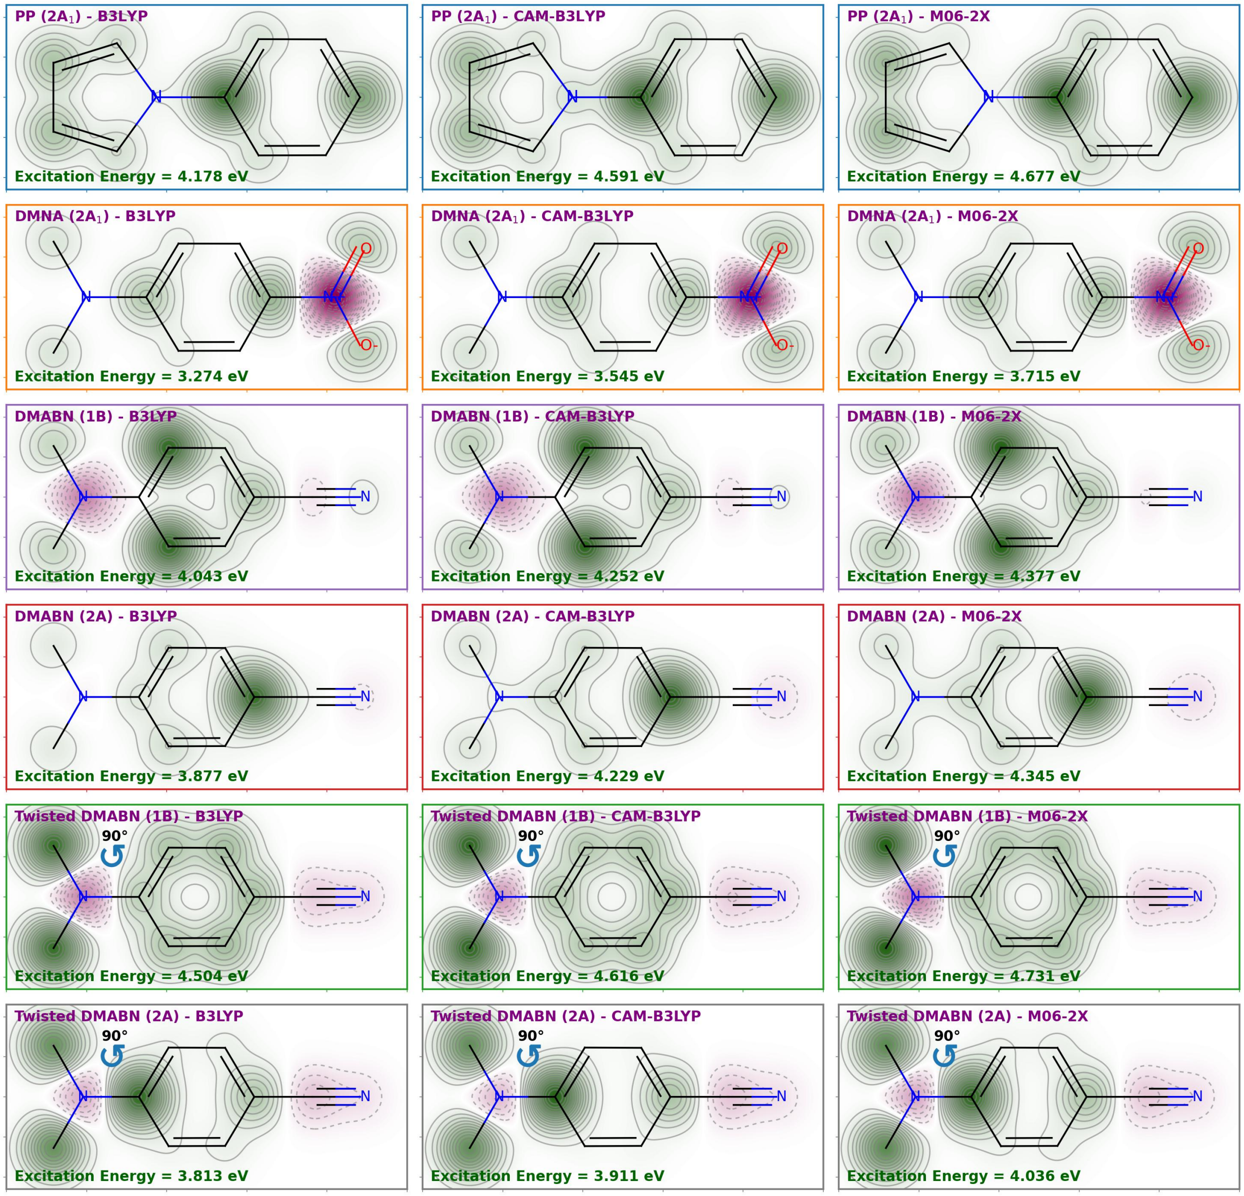


**Figure S3:** Total changes in individual atomic electronic energy contributions along the studied transitions in PP, DMNA, and (twisted) DMABN (in vacuo), as calculated using a selection of DFAs in the aug-pc-1 basis set and a combination of IBOs/IAOs. The colormap is the same as in Fig. S1, and the plots have been (row-wise) normalized for each of the individual transitions.

# 5 Basis Set

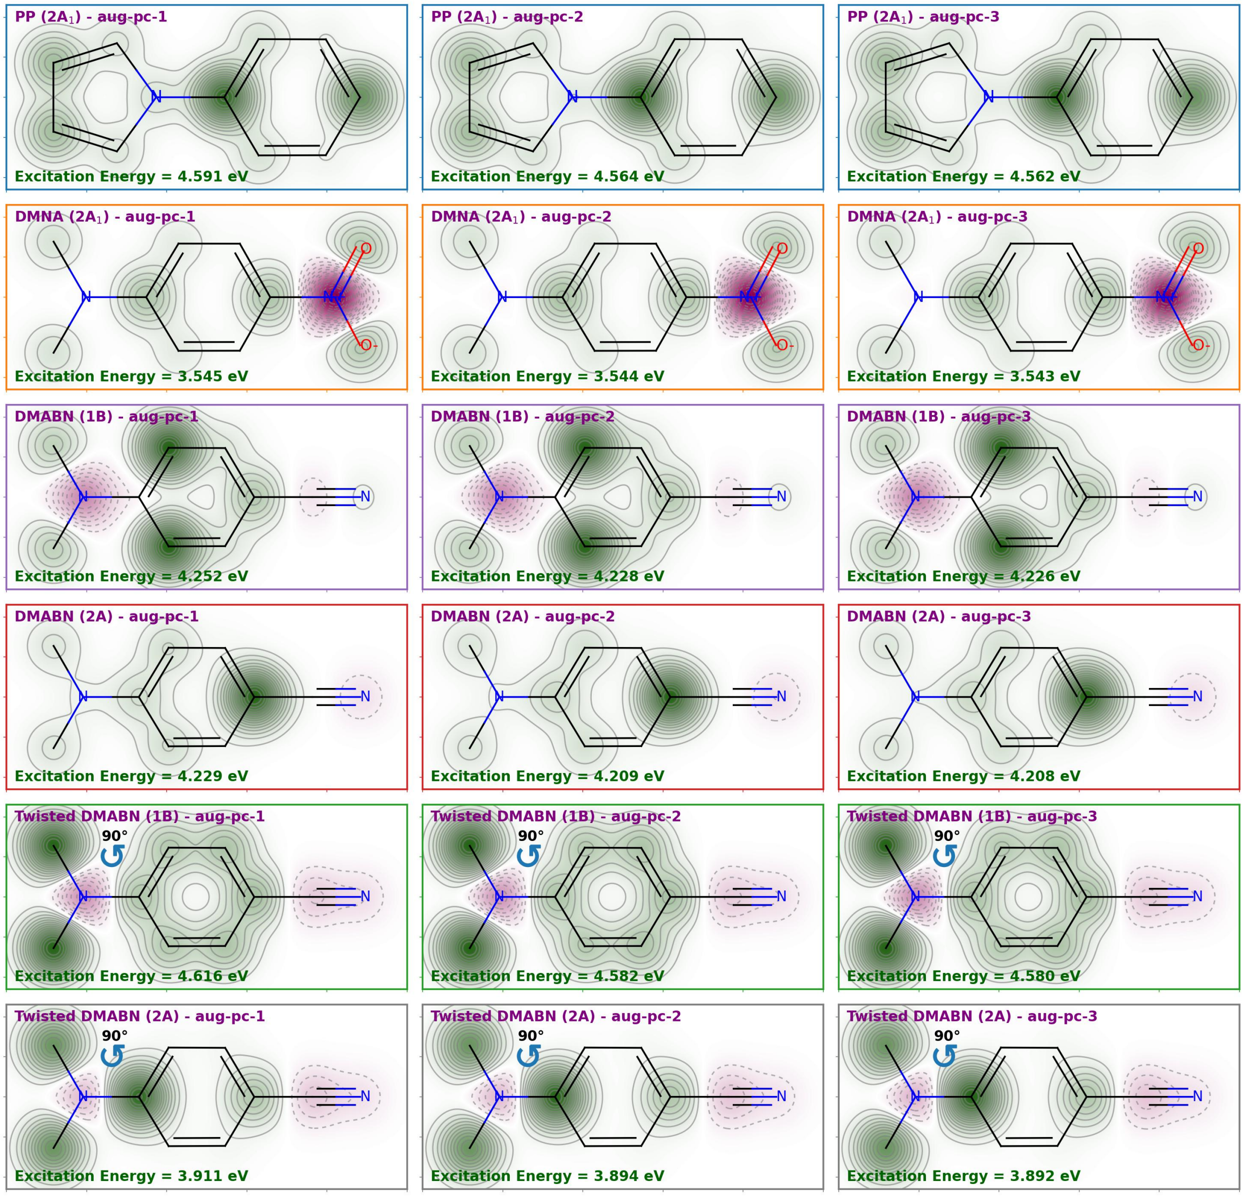


**Figure S4:** Total changes in individual atomic electronic energy contributions along the studied transitions in PP, DMNA, and (twisted) DMABN (in vacuo), as calculated using the CAM-B3LYP *xc* functionals in the aug-pc-*n* family of basis sets and a combination of IBOs/IAOs. The colormap is the same as in Fig. S1, and the plots have been (row-wise) normalized for each of the individual transitions.

# 6 TDDFT

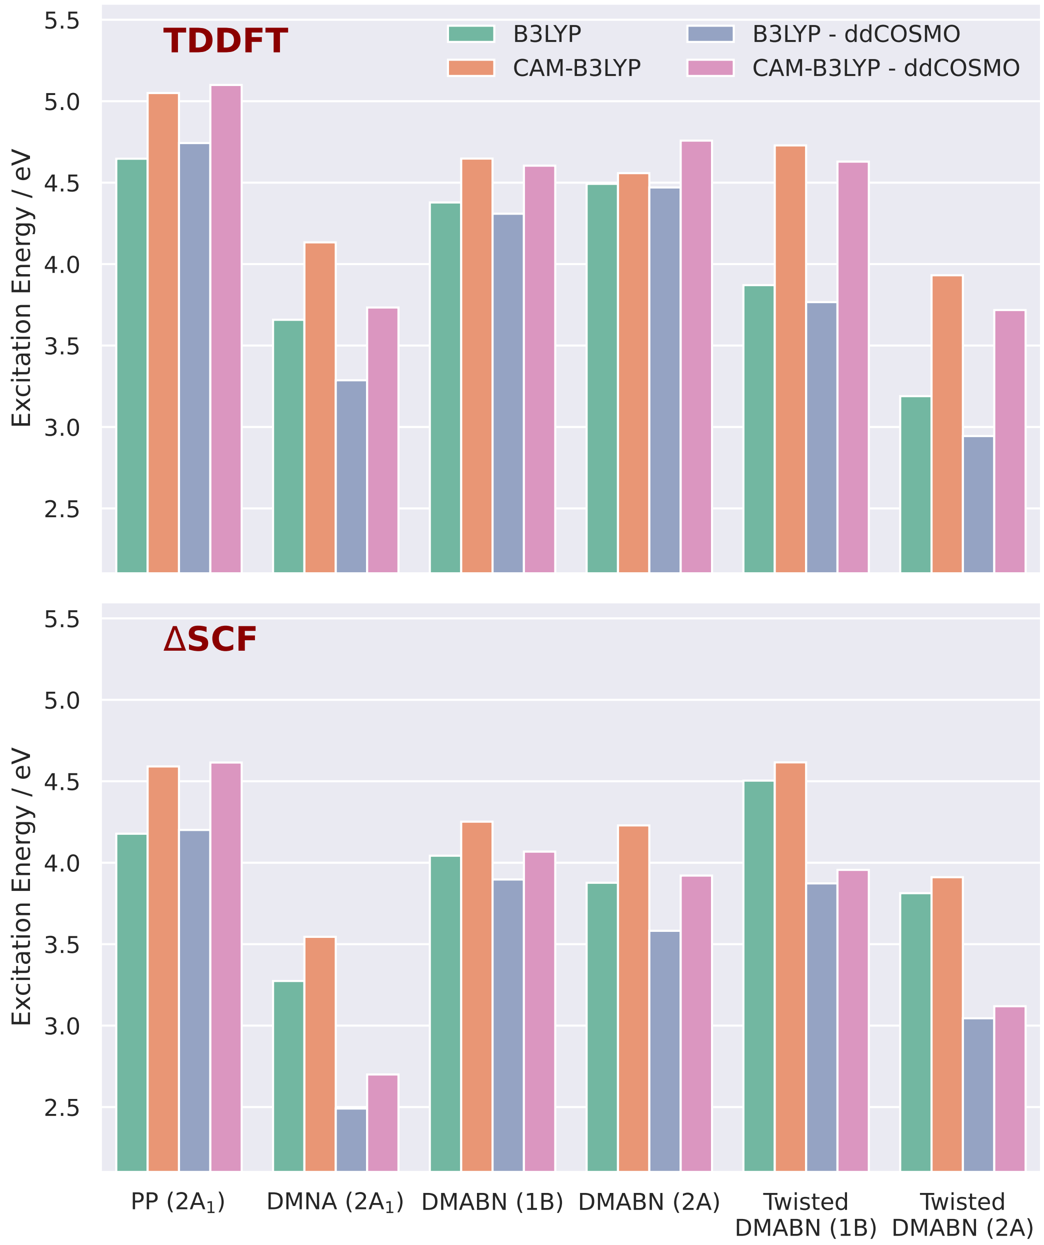


**Figure S5:** Total TDDFT and ΔSCF excitation energies for the studied transitions in PP, DMNA, and (twisted) DMABN (in vacuo or ddCOSMO solution), as calculated using the B3LYP and CAM-B3LYP *xc* functionals in the aug-pc-1 basis set.

# 7 Decomposition Technique

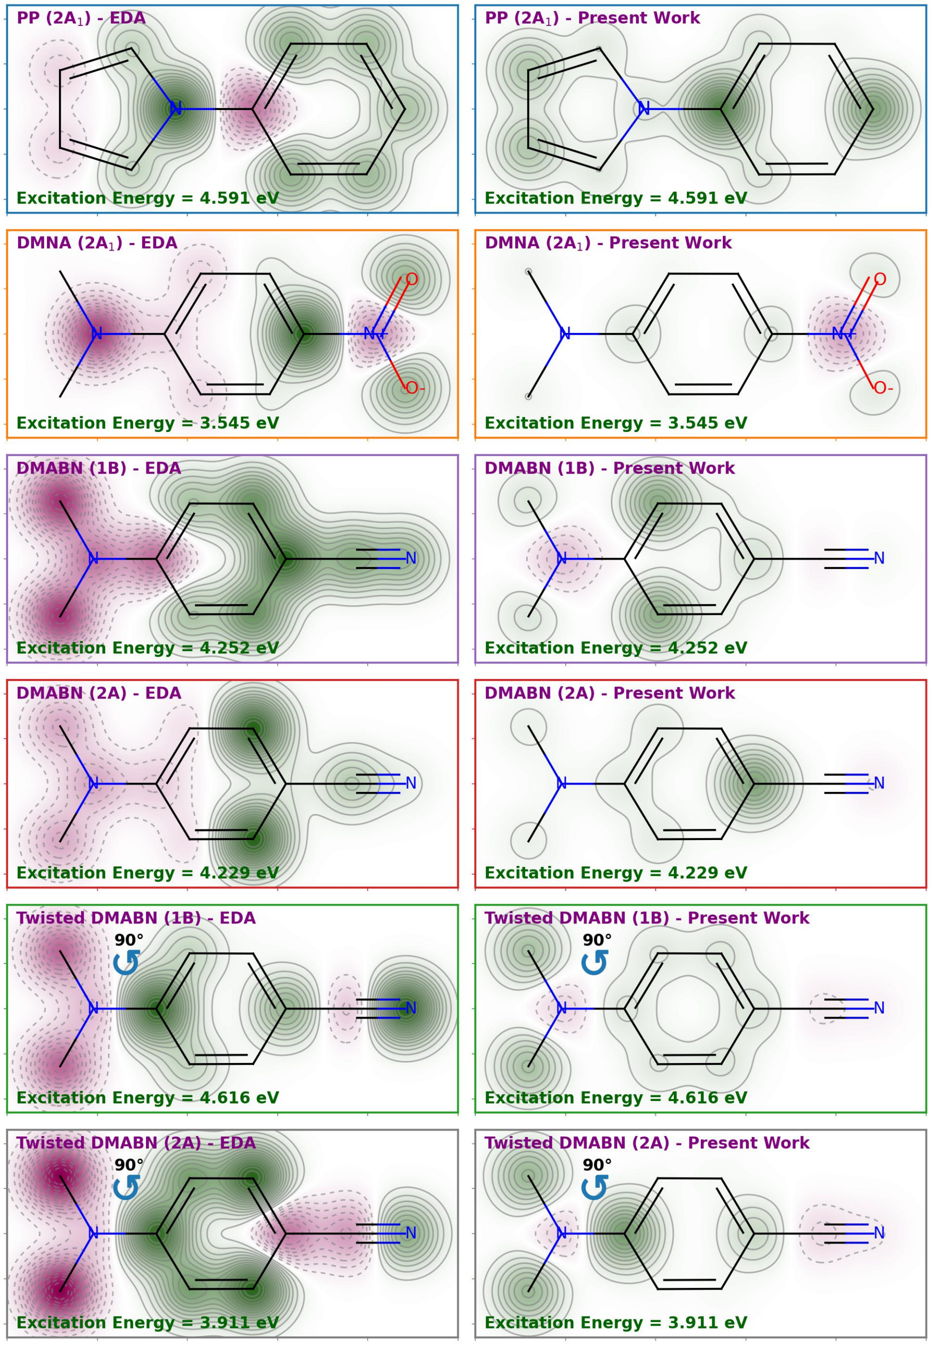


**Figure S6:** Total changes in individual atomic electronic energy contributions along the studied transitions in PP, DMNA, and (twisted) DMABN (in vacuo), as calculated at the CAM-B3LYP/aug-pc-1 level of theory and either the present decompositions (with a combination of IBOs/IAOs) or the EDA scheme. The colormap is the same as in Fig. S1, and the plots have been (row-wise) normalized for each of the individual transitions.

# 8 PP ($2A_1$)

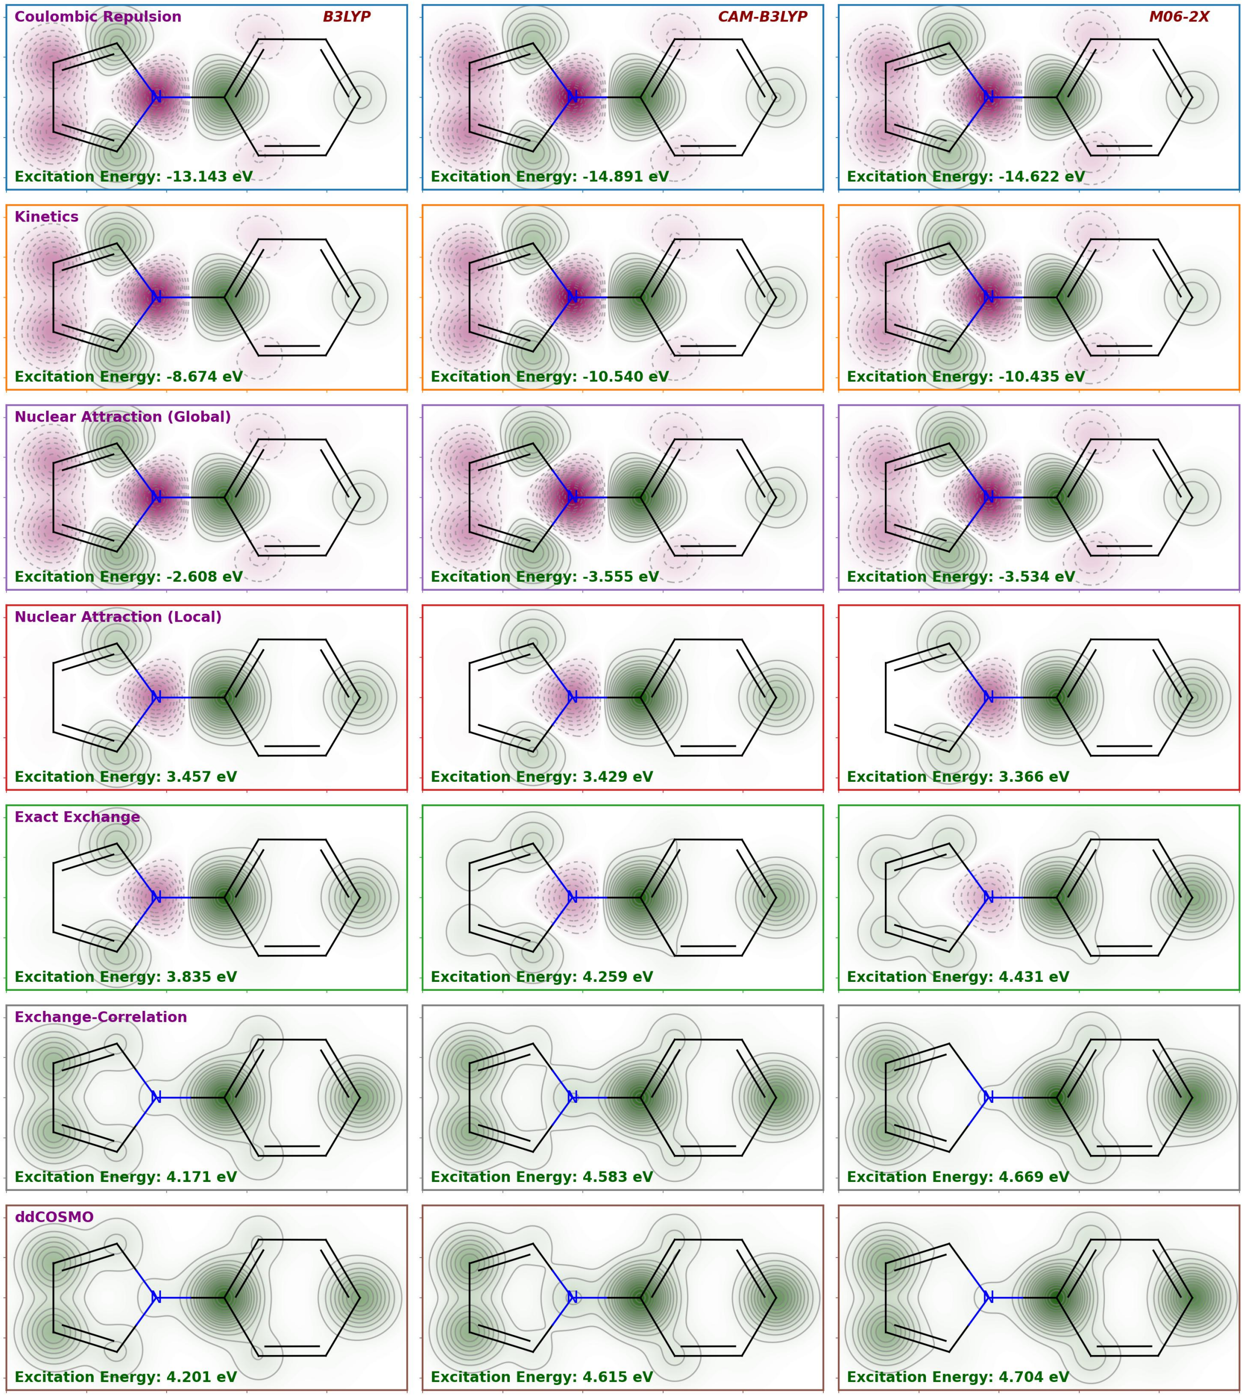


**Figure S7:** Accumulated changes in individual atomic electronic energy contributions along the studied $2A_1$ transition in PP (in ddCOSMO solution), as calculated using the present decompositions, a selection of DFAs, the aug-pc-1 basis set, and a combination of IBOs/IAOs. The colormap is the same as in Fig. S1, and the plots have been (row-wise) normalized for each of the individual contributions.

# 9 DMNA ($2A_1$)

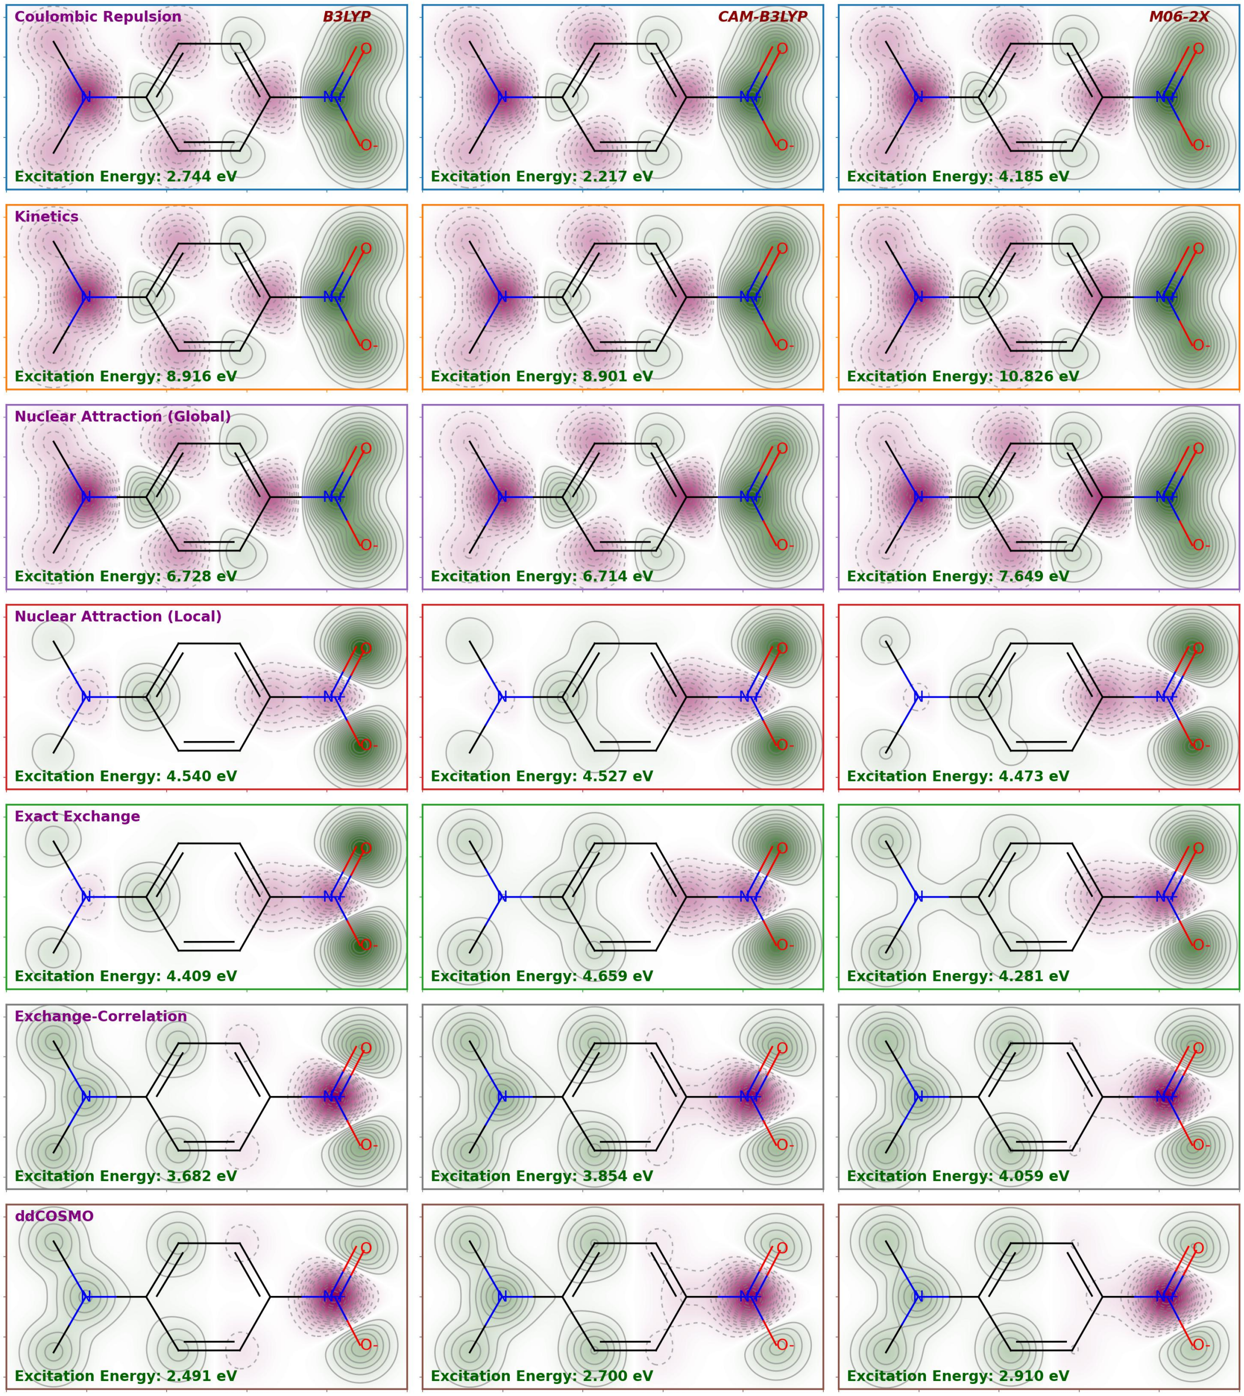


**Figure S8:** Accumulated changes in individual atomic electronic energy contributions along the studied $2A_1$ transition in DMNA (in ddCOSMO solution), as calculated using the present decompositions, a selection of DFAs, the aug-pc-1 basis set, and a combination of IBOs/IAOs. The colormap and normalization are the same as in Fig. S7.

# 10 NA ($2A_1$)

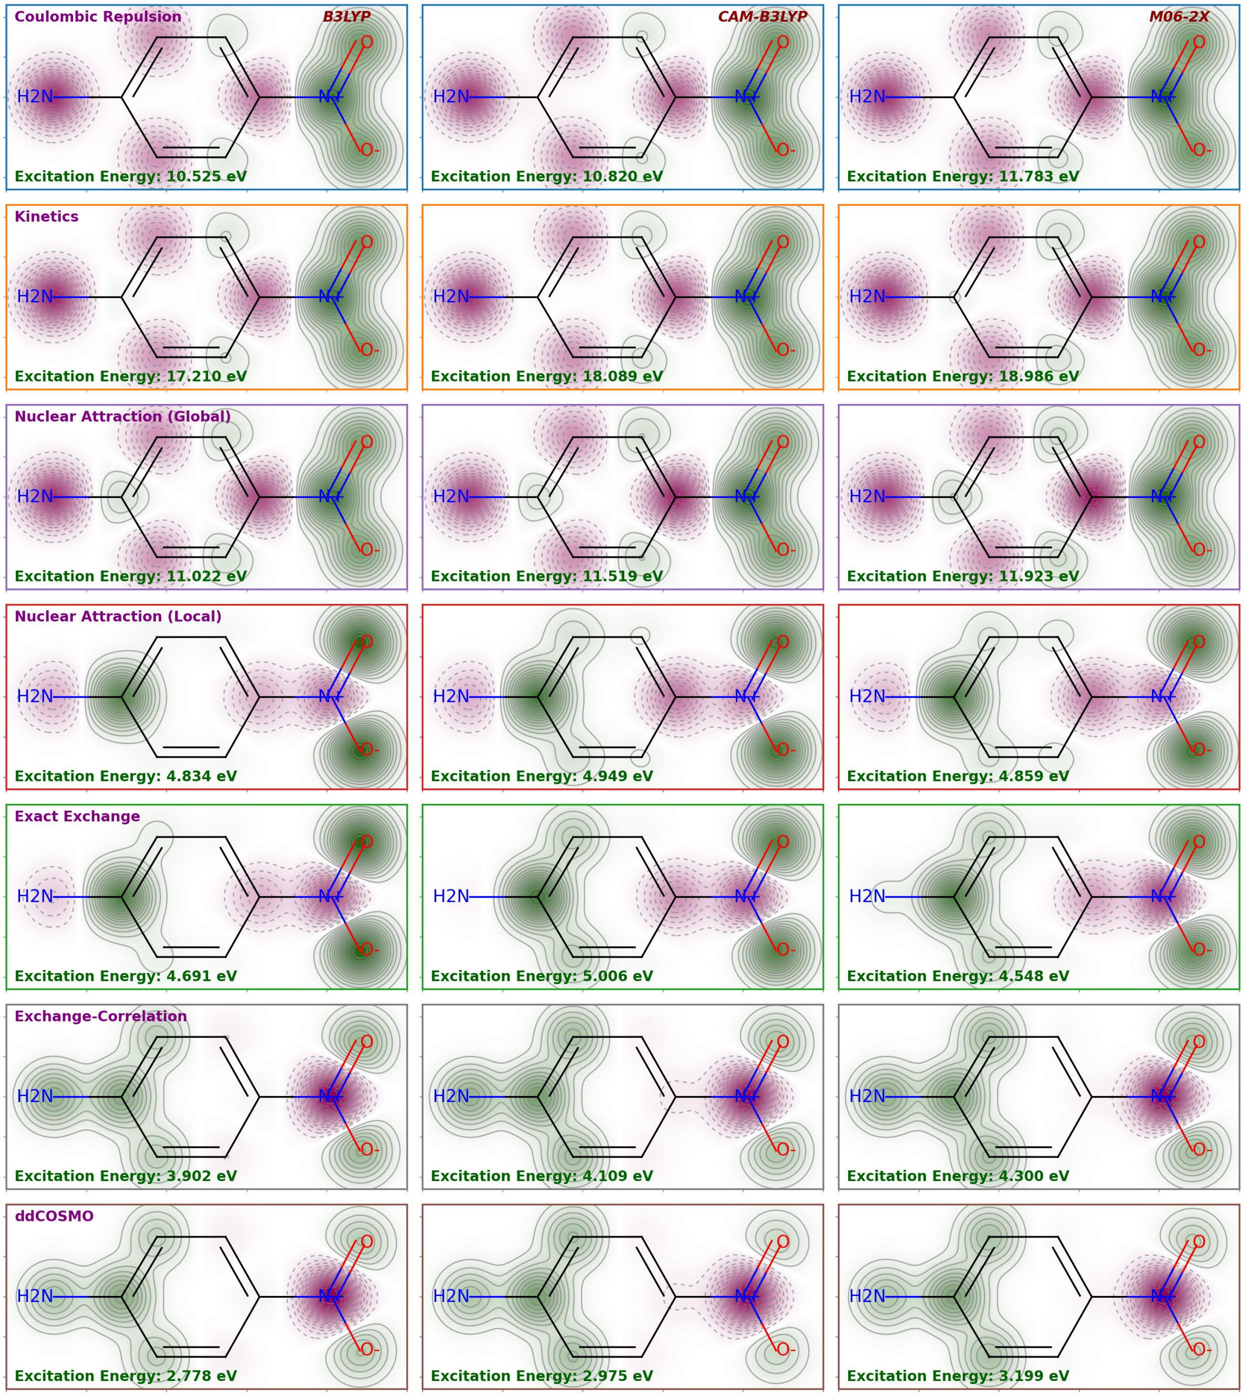


**Figure S9:** Accumulated changes in individual atomic electronic energy contributions along the studied $2A_1$ transition in NA (in ddCOSMO solution), as calculated using the present decompositions, a selection of DFAs, the aug-pc-1 basis set, and a combination of IBOs/IAOs. The colormap and normalization are the same as in Fig. S7.

# 11 DMABN (1B)

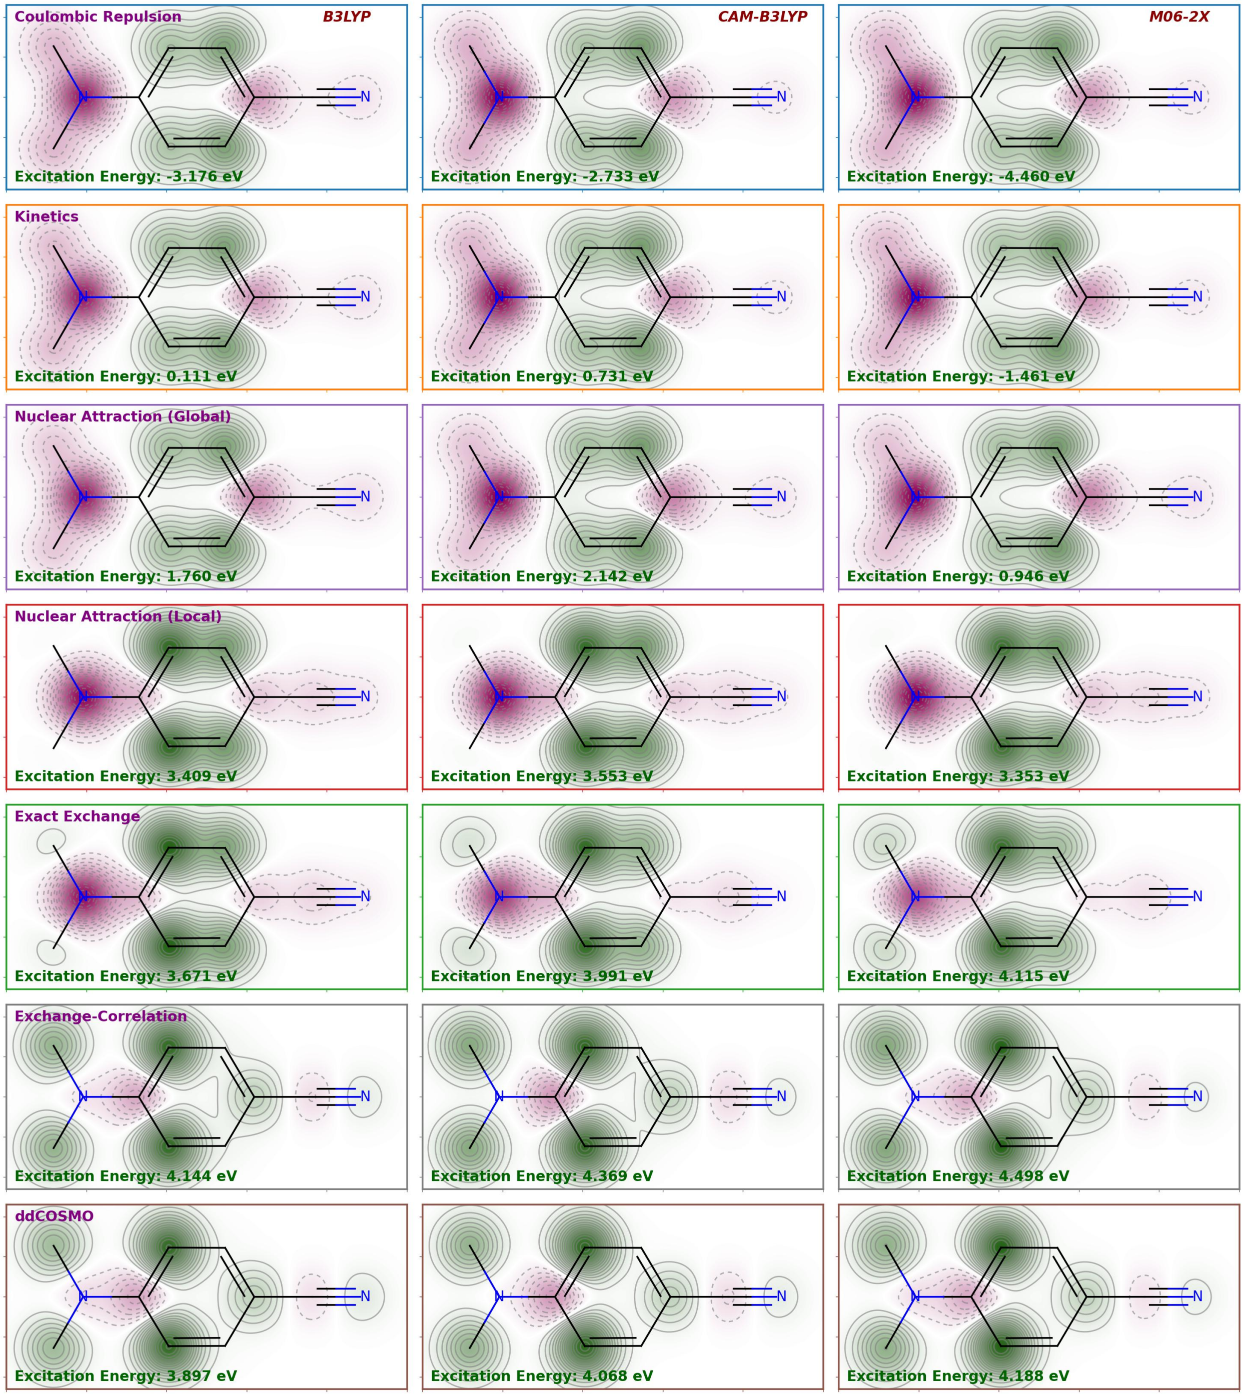


**Figure S10:** Accumulated changes in individual atomic electronic energy contributions along the studied 2A transition in DMABN (in ddCOSMO solution), as calculated using the present decompositions, a selection of DFAs, the aug-pc-1 basis set, and a combination of IBOs/IAOs. The colormap and normalization are the same as in Fig. S7.

# 12 DMABN (2A)

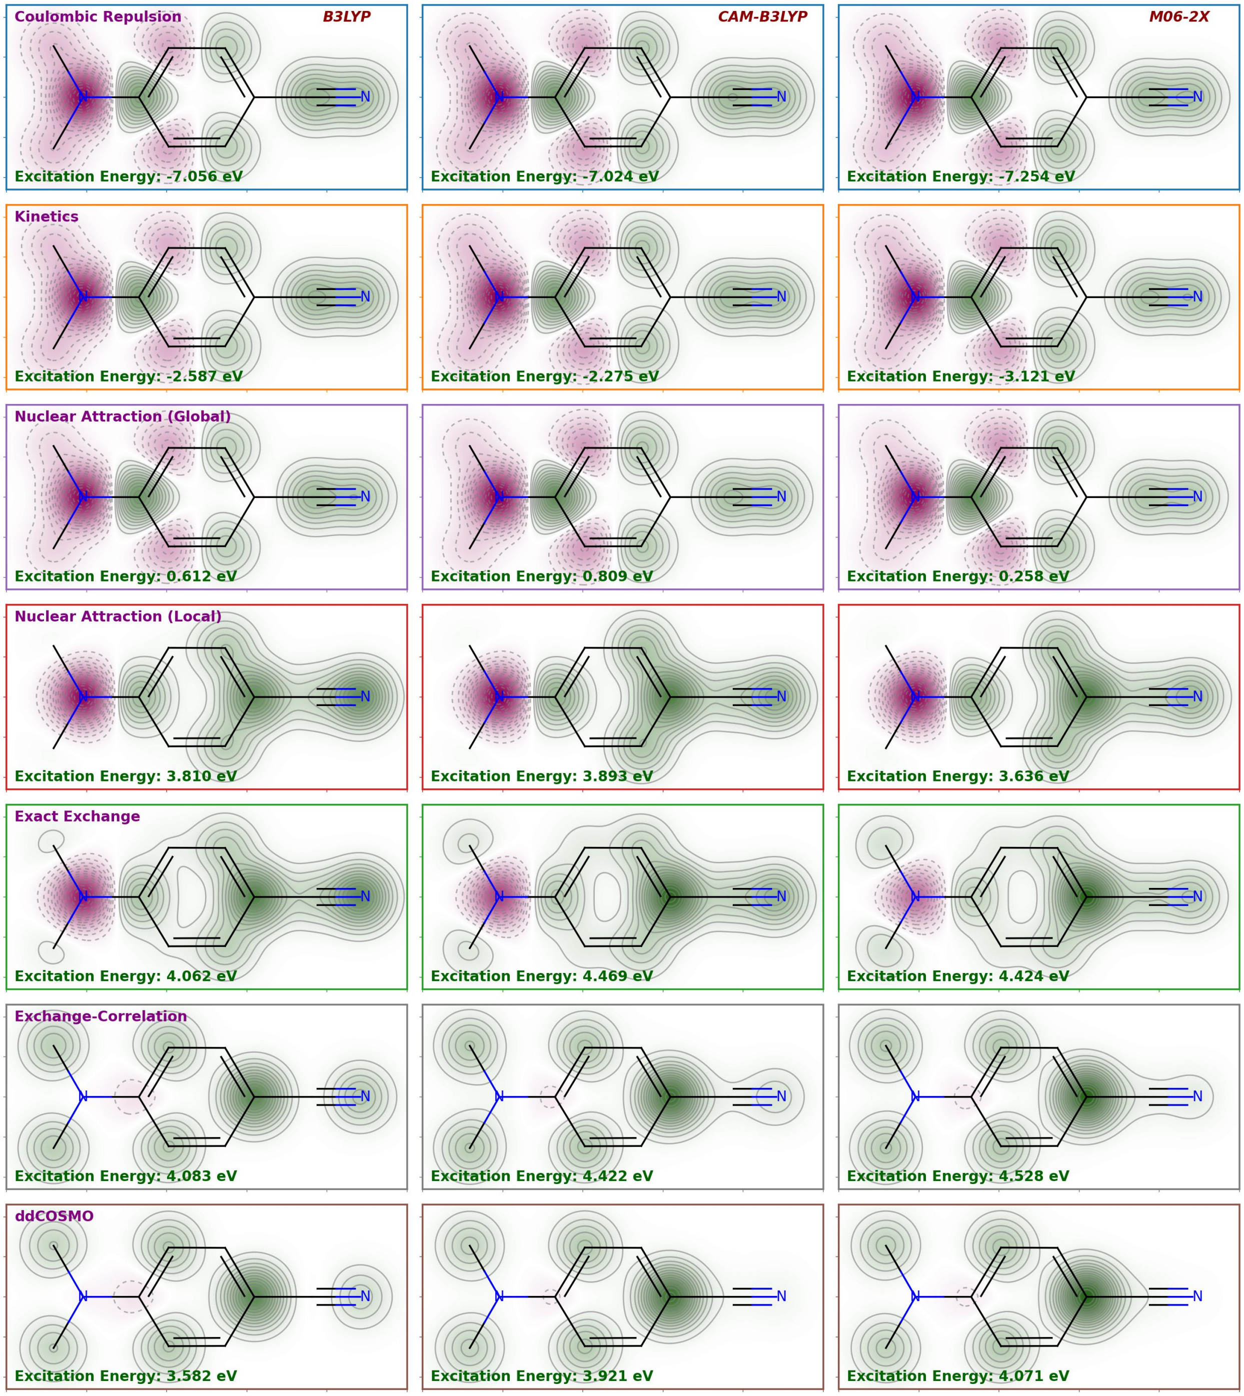


**Figure S11:** Accumulated changes in individual atomic electronic energy contributions along the studied 2A transition in DMABN (in ddCOSMO solution), as calculated using the present decompositions, a selection of DFAs, the aug-pc-1 basis set, and a combination of IBOs/IAOs. The colormap and normalization are the same as in Fig. S7.

# 13 Twisted DMABN (1B)

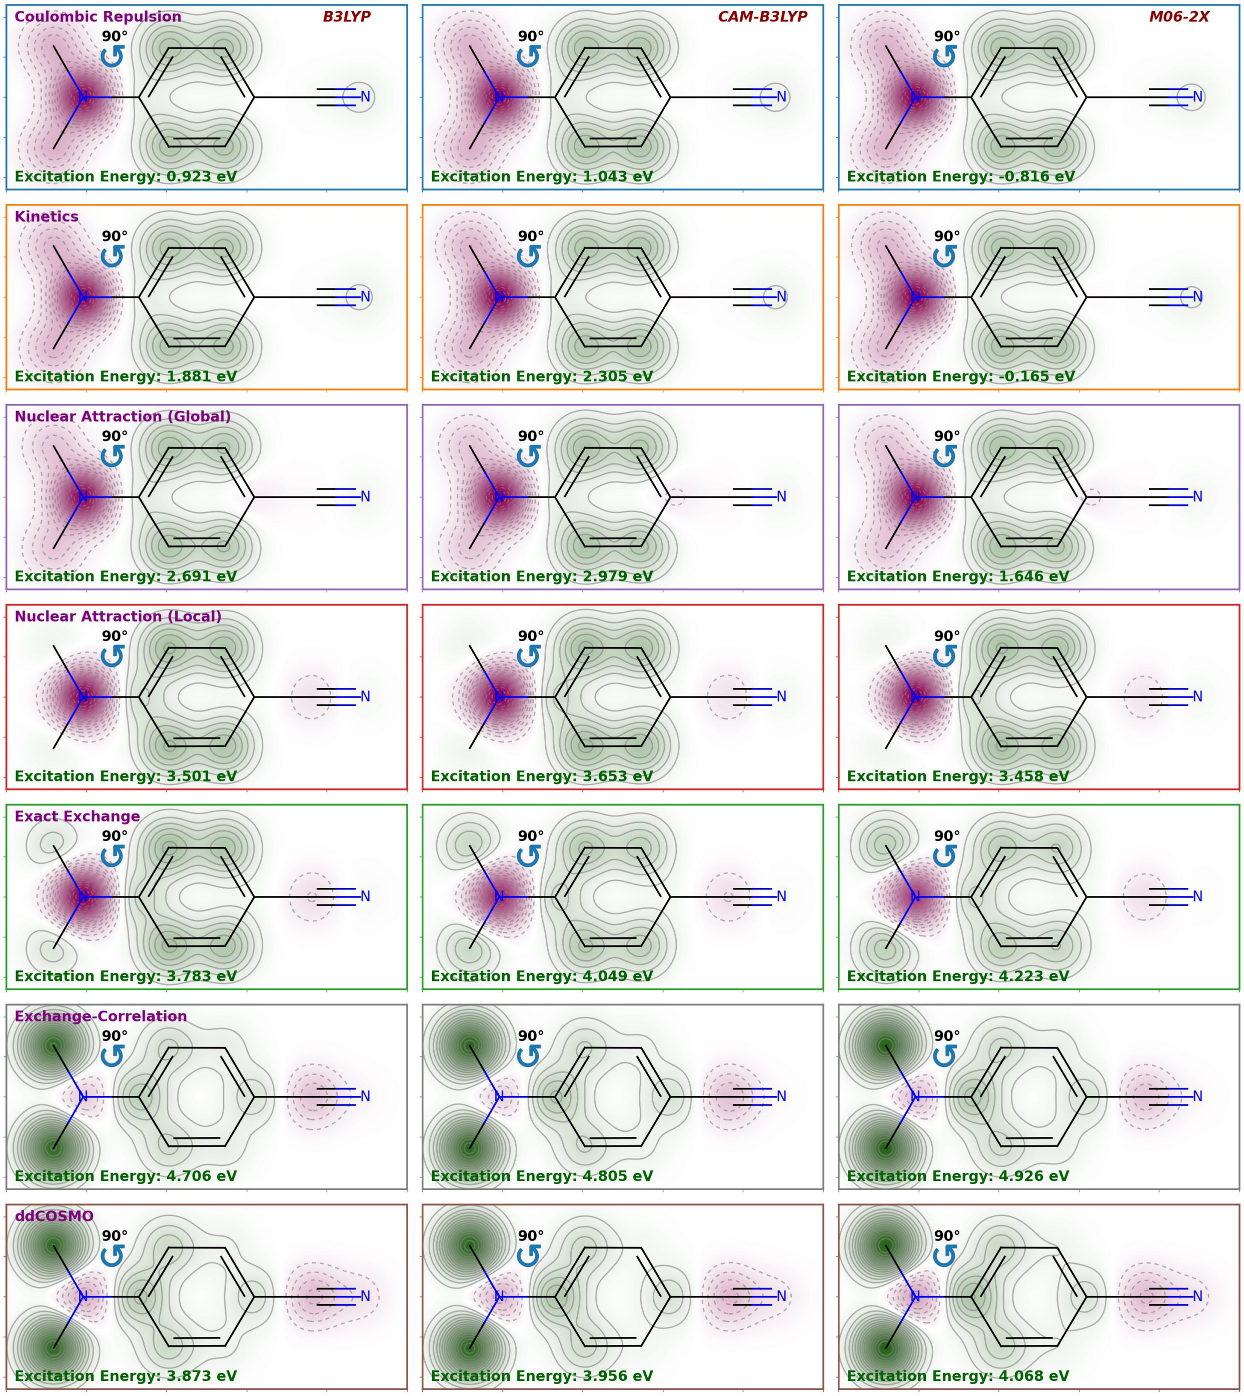


**Figure S12:** Accumulated changes in individual atomic electronic energy contributions along the studied 1B transition in twisted DMABN (in ddCOSMO solution), as calculated using the present decompositions, a selection of DFAs, the aug-pc-1 basis set, and a combination of IBOs/IAOs. The colormap and normalization are the same as in Fig. S7.

# 14 Twisted DMABN (2A)

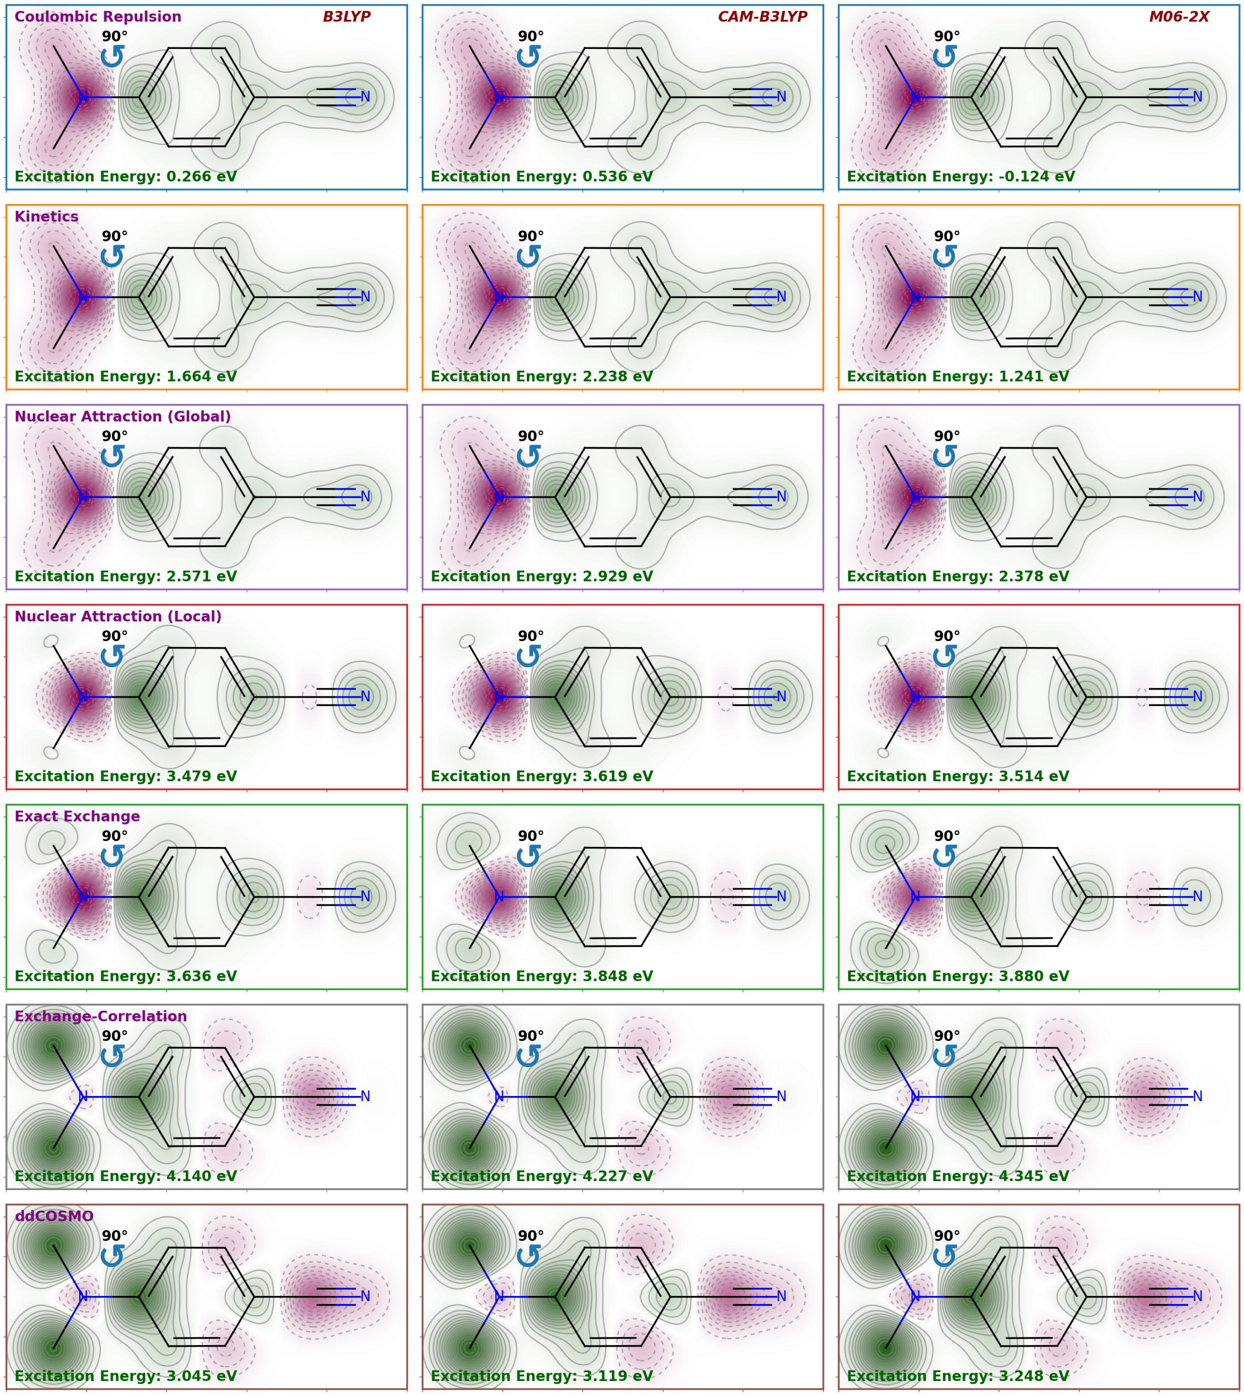


**Figure S13:** Accumulated changes in individual atomic electronic energy contributions along the studied 2A transition in twisted DMABN (in ddCOSMO solution), as calculated using the present decompositions, a selection of DFAs, the aug-pc-1 basis set, and a combination of IBOs/IAOs. The colormap and normalization are the same as in Fig. S7.
